# Supplementary material for: Adaptive Prompting for Continual Relation Extraction: A Within-Task Variance Perspective
Source: arXiv:2412.08285 source file (2025-01-18)
Supplement: Supplementary file 1 [file appendix.tex]

\appendix

\section{Training Framework}

\label{appendix:training_algorithm}

\begin{algorithm}[!t]
\caption{$\mathcal{T}_t$ training process}\label{alg:cap}
\begin{algorithmic}[1]
\Require Training $t$-th dataset $\mathcal{D}_t$, current relation set $\mathcal{R}_t$, history relation set $\hat{\mathcal{R}}_{t-1}$, task-specific Prompt Pool set $\hat{\mathbf{P}}_{t-1}$, generative model set $\hat{\mathbf{G}}_{t-1}$
\Ensure Task-specific Prompt Pool set $\hat{\mathbf{P}}_{t}$, generative model set $\hat{\mathbf{G}}_{t}$, relation classifier $g_\phi$, task predictor $\hat{g}_\psi$
\STATE Initialize $\mathbf{P}_t$ 
\FOR{$e_{id} \gets 1$ \textbf{to} $training\_epoch$}
\FOR{$each$ mini batch $\boldsymbol{x}_{B} \in \mathcal{D}_t$}
\STATE Update $\mathbf{P}_t$ and $g_{\phi}$ on $\boldsymbol{x}_{B}$  \COMMENT{Eq.\eqref{eq:prompt-pool-learning-loss}}

\ENDFOR
\ENDFOR
\STATE $\hat{\mathcal{R}}_{t} \gets \hat{\mathcal{R}}_{t-1} \cup \mathcal{R}_t$
\STATE $\hat{\mathbf{P}}_{t} \gets \hat{\mathbf{P}}_{t-1} \cup \mathbf{P}_t$
\STATE $\mathbf{G}_{z_t} \gets \emptyset$, $\mathbf{G}_{q_t} \gets \emptyset$ \COMMENT{$t$-th GMMs set}
\FOR{$each$  $r \in \mathcal{R}_t$}
\STATE $\boldsymbol{x}^r \gets \mathcal{D}^r_t$
\STATE $\mathbf{G}_{z_t} \cup= \mathbf{GMM}(z(\boldsymbol{x}^r, \mathbf{P}_t))$
\STATE $\mathbf{G}_{q_t} \cup= \mathbf{GMM}(q(\boldsymbol{x}^r))$
\ENDFOR
\STATE $\hat{\mathbf{G}}_{z_t} \gets \hat{\mathbf{G}}_{z_{t-1}} \cup \mathbf{G}_{z_t}$
\STATE $\hat{\mathbf{G}}_{q_t} \gets \hat{\mathbf{G}}_{q_{t-1}} \cup \mathbf{G}_{q_t}$
\STATE $\mathcal{D'}_{z} \gets \emptyset$, $\mathcal{D'}_{q} \gets \emptyset$ \COMMENT{Pseudo Datasets}
\FOR{$each$ $r \in \hat{\mathcal{R}}_t$}
\STATE $\mathcal{D'}_{z} \gets \mathcal{D'}_{z} \cup Sample(\mathbf{G}^r_z)$
\STATE $\mathcal{D'}_{q} \gets \mathcal{D'}_{q} \cup Sample(\mathbf{G}^r_{q})$
\ENDFOR
\FOR{$each$ mini batch $z_{B} \in \mathcal{D'}_z$} \STATE Update $g_\phi$ via $\mathcal{L}_{CE}$ on $z_{B}$
\ENDFOR
\FOR{$each$ mini batch ${q}_{B} \in \mathcal{D'}_{q}$}
\STATE Update $\hat{g}_\psi$ via $\mathcal{L}_{CE}$ on ${q}_{B}$
\ENDFOR
\STATE \textbf{Return} $\hat{\mathbf{P}}_{t}, \hat{\mathbf{G}}_{t}, \phi, \psi$
\end{algorithmic}
\end{algorithm}

\begin{figure*}
    \vspace{-1.5cm}
    \includegraphics[scale=0.29]{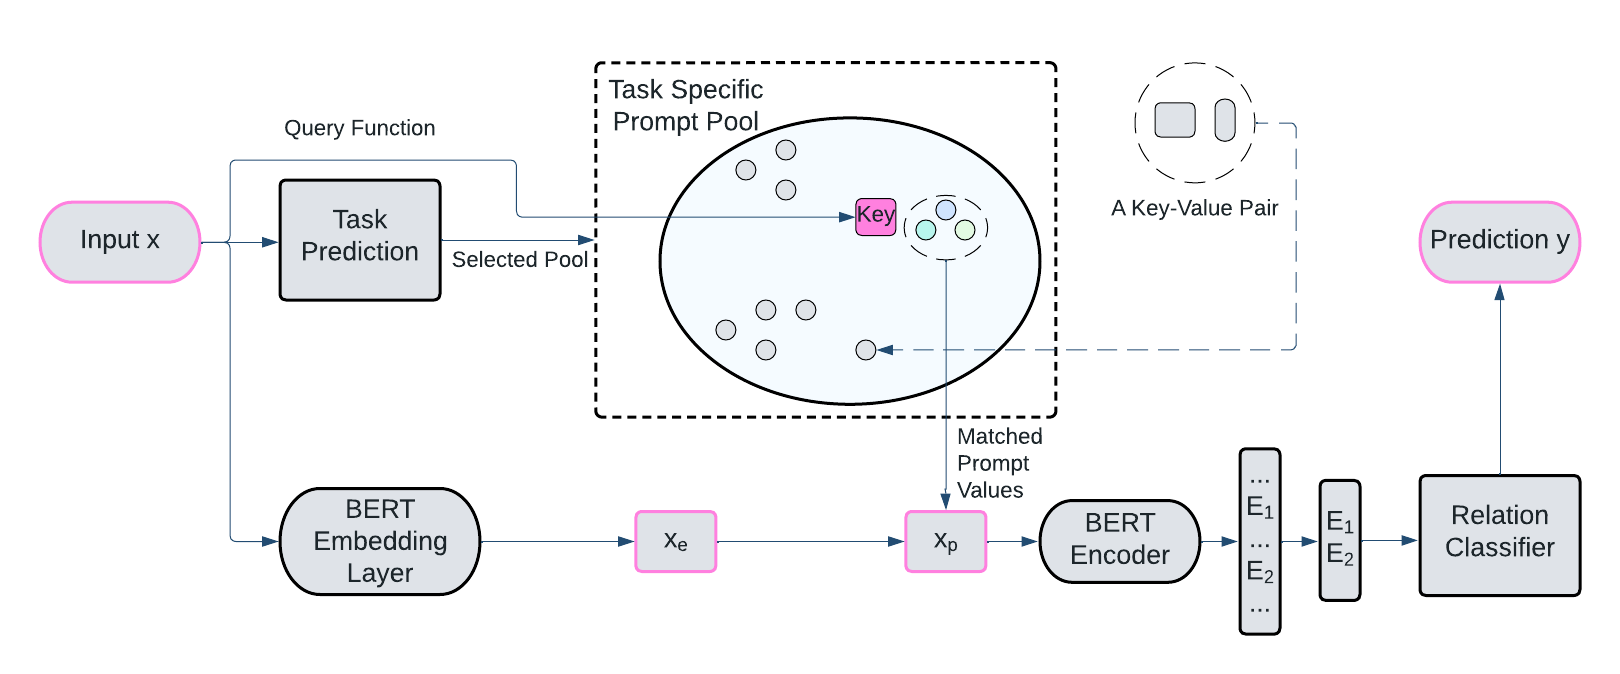}
    \captionsetup{justification=justified, singlelinecheck=false}
    \captionsetup{skip=-7.5pt}
    \caption{\textbf{Data Flow Diagram}: Initially, the Task Predictor predicts the task identity of the input $\boldsymbol{x}$, enabling the selection of the corresponding Prompt Pool. Subsequently, the input $\boldsymbol{x}$ queries this Prompt Pool to identify prompts whose corresponding keys are closest to the $query \ q(\xbm)$. The chosen prompt is then prepended to the embedded input $\boldsymbol{x}_e$, creating the prompted input $\boldsymbol{x}_p$. The combined $\boldsymbol{x}_p$ is fed into the BERT Encoder, where the two embeddings corresponding to the positions of the entities $E_1$ and $E_2$ are concatenated. Finally, the resulting concatenated embedding is passed to the Class Classifier, which predicts the relation label $y$ of the input $\boldsymbol{x}$.}
    \label{fig:data-flow-diagram}
\end{figure*}

\textbf{(1) Prompt Pool learning FOR a new task} (line 1 $\sim$ 6):  When the data FOR the $t$-th task arrives, consisting of dataset $\mathcal{D}_t$ and its corresponding relation set $\mathcal{R}_t$, a task-specific Prompt Pool $\mathbf{P}_t$ is initialized and employed to be associated with the $t$-th task. This Prompt Pool is trained alongside a simple relation classifier $g_\phi$ to classify the relations in $\mathcal{R}_t$ based on the dataset $\mathcal{D}_t$. Throughout this learning process, the pre-trained BERT model remains frozen, while knowledge pertaining to relations in $\mathcal{R}_t$ is acquired and stored in $\mathbf{P}_t$.

\textbf{(2) Generative Models} (line 7 $\sim$ 13): FOR each new relation $r \in \mathcal{R}_t$ trained in Step 1, we utilize two Gaussian Mixture Models (GMMs): $\mathbf{G}^r_{q}$ and $\mathbf{G}^r_z$. These models serve to preserve the distribution of high-dimensional representations of all the samples labeled by $r$. Specifically, $\mathbf{G}^r_{q}$ captures the distribution of the unprompted relation representations, while $\mathbf{G}^r_z$ learns the distribution of prompted relation representations. We refer to the collections of GMMs representing the $t$-th task as $\mathbf{G}_t = \{\mathbf{G}_{q_t}, \mathbf{G}_{z_t}\}$. Furthermore, we denote the collections of GMMs learned up to the $t$-th task as $\hat{\mathbf{G}}_t = \{\hat{\mathbf{G}}_{q_t}, \hat{\mathbf{G}}_{z_t}\}$. These GMMs will be utilized to generate inputs FOR training classifiers. The purpose of generating the $query$ is to determine the task identity, while the generated $z$ is employed FOR relation classification, as outlined in Step 3 below.

\textbf{(3) Training the Task Predictor and Relation Classifier} (line 14 $\sim$ 21): To classify an unlabeled sample $\boldsymbol{x}$, we employ two distinct neural networks: the task predictor, denoted as $\hat{g}_\psi$, and the relation classifier, referred to as $g_\phi$. $\hat{g}_\psi$ utilizes the $query$ representations derived from $\hat{\mathbf{G}}_{q_t}$ as its input and focuses on predicting the task identity of $\boldsymbol{x}$. On the other hand, $g_\phi$ operates on the $z$ representations sampled from $\hat{\mathbf{G}}_{z_t}$ to accurately classify the relation class $r \in \hat{\mathcal{R}}_t$ of the samples.

During the training process, our main focus lies on Steps 1 and 2. Step 3 is specifically utilized FOR evaluating the model and does not directly impact the training procedure. See Figure~\ref{fig:data-flow-diagram} FOR the data flow diagram at inference.

\section{Experimental Details}
\label{appendix:exp}

\textbf{Datasets.} \textbf{Datasets.} We evaluate WAVE-CRE and all baselines on two datasets: TACRED \cite{zhang2017tacred} and FewRel \cite{han-etal-2018-fewrel}. FewRel contains 80 relation types with a total of 56,000 samples. Following the configurations outlined in \cite{wang-etal-2019-sentence}, we split it into 10 non-overlapping groups FOR simulating 10 sequential training tasks. The TACRED dataset is an imbalanced dataset FOR CRE, containing 42 relations and 106,264 samples.  We adopt the experimental settings proposed by \cite{cui-etal-2021-refining}, similar to the CRE approach presented in \cite{zhao-etal-2022-consistent}.

\textbf{Baselines.} As we have already discussed L2P \cite{wang2022learning}, DualPrompt \cite{wang2022dualprompt}, and HiDe-Prompt \cite{wang2023hide} in the main paper, we focus on the remaining baselines here. Briefly, \textbf{CODA-Prompt} \cite{smith2023coda} expands the prompt pool across tasks and perFORms a weighted summation of the prompt pool using attention factors. \textbf{EPI} \cite{epi2023} applied a parameter isolation strategy with a non-parametric method to load the correct parameters at test time. \textbf{EA-EMR} \citep{wang-etal-2019-sentence} introduced a technique that combines memory replay and embedding alignment to address catastrophic FORgetting. \textbf{CML} \citep{wu2021curriculum} presented a curriculum-meta learning approach to tackle order-sensitivity and catastrophic FORgetting in CRE. \textbf{EMAR + BERT} \citep{han-etal-2020-continual} proposed a method based on memory activation and reconsolidation to preserve prior knowledge. \textbf{RP-CRE} \citep{cui-etal-2021-refining} utilized a memory network to refine sample embeddings with relation prototypes, aiming to prevent catastrophic FORgetting. \textbf{CRECL} \citep{hu2022improving} combined a classification network and a prototypical contrastive network to alleviate the problem of catastrophic FORgetting. \textbf{CRL} \citep{zhao-etal-2022-consistent} employed a contrastive replay mechanism and knowledge distillation to maintain learned knowledge. \textbf{EMAR+ACA} \citep{wang-etal-2022-learning-robust} enhances CRE models by using a data augmentation mechanism to enhance the robustness of the learned model. \textbf{CRE-DAS} \cite{zhao2023improving} employed memory-insensitive relation prototypes and memory augmentation to overcome overfitting; they also introduced integrated training and focal knowledge distillation to enhance perFORmance on analogous relations. \textbf{CDec+ACA} \cite{xia2023enhancing} proposed a classifier decomposition framework to address representation biases by promoting robust representation learning while preserving previous knowledge.

\textbf{Training Details.} In this work, we used a single NVIDIA A100 FOR all methods. To tune the proposed model, we choose $gmm\_num\_components$ from [1, 3, 5], $encoder\_epochs$ from [10, 20, 50], $prompt\_pool\_lr$ from [$2 \times 10^{-5}$, $5 \times 10^{-5}$, $1 \times 10^{-4}$], $classifier\_epochs$ from [100, 300, 500]. All other hyper-parameters will be set as default as in the work of \citet{zhao-etal-2022-consistent}. We tune the hyper-parameters FOR the proposed model using random search. All the hyper-parameters are selected based on the accuracy on both the FewRel and TACRED test sets, as each dataset has its own set of optimal hyper-parameters. Our proposed model has in total 114M parameters. As we freeze the BERT model, the number of learnable parameters is thus only 3.8M. Training on the FewRel dataset took approximately 7 hours, while for the TACRED dataset, it took approximately 3 hours for our method.

\textbf{Evaluation Metrics.}  We use the same perFORmance measures (mean accuracy on 5 different random seeds) as in prior work \cite{zhao-etal-2022-consistent} FOR fair comparison.
